# Supplementary material for: HALO: Fault-Tolerant Safety Architecture For High-Speed Autonomous Racing
Source: arXiv:2503.10341 source file (2025-03-13)
Supplement: Supplementary file 1 [file Appendix_A.tex]

\label{sec:appendix_a}

\begin{table*}[p]
\begin{tabular}{c|c|c|c|c}
    \textbf{Node} & \textbf{Topic} & \textbf{I/O Type} & \textbf{Failure Type} & \textbf{HALO Safety Node} \\
    \hline
    Long Control & /joystick/command & Input & Data Health & Graceful Stop \\
     & /graceful\_stop/long\_control & Input & Node Health & Node Health Monitor \\
     & /raptor\_dbw\_interface/wheel\_speed\_report & Input & Data Health & None \\
     & /heartbeat/long\_control & Output & Node Health & Node Health Monitor \\
     & /joystick/accelerator\_cmd & Output & Data Health & SSC Interface \\
     & /joystick/brake\_cmd & Output & Data Health & SSC Interface \\
     & /joystick/gear\_cmd & Output & Data Health & SSC Interface \\
    \hline
    Path Tracker & /joystick/command & Input & Data Health & Graceful Stop \\
     & /switch\_path & Input & Behavioral-Safety & Path Tracker \\
     & /vehicle/uva\_odometry & Input & Data Health & Graceful Stop \\
     & /raptor\_dbw\_interface/wheel\_speed\_report & Input & Data Health & None \\
     & /heartbeat/path\_tracker & Output & Node Health & Node Health Monitor \\
     & /joystick/steering\_cmd & Output & Data Health & SSC Interface \\
    \hline
\end{tabular}
\caption{\label{table:control_module}Control Module inputs and outputs.}
\end{table*}

\begin{table*}[p]
\begin{tabular}{c|c|c|c|c}
    \textbf{Node} & \textbf{Topic} & \textbf{I/O Type} & \textbf{Failure Type} & \textbf{HALO Safety Node} \\
    \hline
    GPS Top & /novatel\_top/bestpos & Output & & \\
     & /novatel\_top/raw\_imu & Output & & \\
    \hline
    GPS Bottom & /novatel\_bottom/bestpos & Output & & \\
     & /novatel\_bottom/raw\_imu & Output & & \\
    \hline
    Map-Baselink Top & /novatel\_top/bestpos & Input & & \\
     & /novatel\_top/dyntf\_odom & Output & Data Health & Topic Multiplexer \\
    \hline
    Map-Baselink Bottom & /novatel\_bottom/bestpos & Input & & \\
     & /novatel\_bottom/dyntf\_odom & Output & Data Health & Topic Multiplexer \\
    \hline
    Convert IMU Top & /novatel\_top/raw\_imu & Input & & \\
     & /corrected\_imu\_top & Output & & \\
    \hline
    Convert IMU Bottom & /novatel\_bottom/raw\_imu & Input & & \\
     & /corrected\_imu\_bottom & Output & & \\
    \hline
    EKF & /novatel\_top/dyntf\_odom & Input & Data Health & Topic Multiplexer \\
     & corrected\_imu\_top & Input & & \\
     & /novatel\_bottom/dyntf\_odom & Input & Data Health & Topic Multiplexer \\
     & corrected\_imu\_bottom & Input & & \\
     & /wheel & Input & & \\
     & /odometry\_filtered & Output & Data Health & Topic Multiplexer \\
    \hline
    Topic Multiplexer & /novatel\_top/dyntf\_odom & Input & Data Health & Topic Multiplexer \\
     & /novatel\_bottom/dyntf\_odom & Input & Data Health & Topic Multiplexer \\
     & /odometry\_filtered & Input & Data Health & Topic Multiplexer \\
     & /raptor\_dbw\_interface/rc\_to\_ct & Input & Data Health & Topic Multiplexer \\
     & /raptor\_dbw\_interface/rc\_to\_ct\_bs & Input & Data Health & Topic Multiplexer \\
     & /raptor\_dbw\_interface/wheel\_speed\_report & Input & & \\
     & /vehicle/uva\_odometry & Output & Data Health & Graceful Stop \\
     & /vehicle/no\_odom & Output & Data Health & Graceful Stop \\
     & /vehicle/rc\_to\_ct\_info & Output & Data Health & Topic Multiplexer \\
     & /heartbeat/topic\_multiplexer & Output & Node Health & Node Health Monitor \\
     \hline
\end{tabular}
\caption{\label{table:localization_module}Localization Module inputs and outputs.}
\end{table*}

\begin{table*}[p]
\begin{tabular}{c|c|c|c|c}
    \textbf{Node} & \textbf{Topic} & \textbf{I/O Type} & \textbf{Failure Type} & \textbf{HALO Safety Node} \\
    \hline
    SSC Interface & /joystick/command & Input & Data Health & Graceful Stop \\
     & /vehicle/uva\_odometry & Input & Data Health & Graceful Stop \\
     & /vehicle/emergency\_joystick & Input & Data Health & None \\
     & /vehicle/emergency\_heartbeat & Input & Data Health & Graceful Stop \\
     & /heartbeat/diagnostics & Input & Node Health & Graceful Stop \\
     & /joystick/accelerator\_cmd & Input & Data Health & SSC Interface \\
     & /joystick/brake\_cmd & Input & Data Health & SSC Interface \\
     & /joystick/gear\_cmd & Input & Data Health & SSC Interface \\
     & /joystick/steering\_cmd & Input & Data Health & SSC Interface \\
     & /raptor\_dbw\_interface/misc\_report\_do & Input & Data Health & None \\
     & /raptor\_dbw\_interface/wheel\_speed\_report & Input & Data Health & None \\
     & /raptor\_dbw\_interface/accelerator\_pedal\_cmd & Output & Data Health & SSC Interface \\
     & /raptor\_dbw\_interface/brake\_cmd & Output & Data Health & SSC Interface \\
     & /raptor\_dbw\_interface/gear\_cmd & Output & Data Health & SSC Interface \\
     & /raptor\_dbw\_interface/steering\_cmd & Output & Data Health & SSC Interface \\
    \hline
    Raptor DBW Node & /raptor\_dbw\_interface/accelerator\_pedal\_cmd & Input & Data Health & SSC Interface \\
     & /raptor\_dbw\_interface/brake\_cmd & Input & Data Health & SSC Interface \\
     & /raptor\_dbw\_interface/gear\_cmd & Input & Data Health & SSC Interface \\
     & /raptor\_dbw\_interface/steering\_cmd & Input & Data Health & SSC Interface \\
     & /raptor\_dbw\_interface/wheel\_speed\_report & Output & & \\
     & /raptor\_dbw\_interface/rc\_to\_ct & Output & Data Health & Topic Multiplexer \\
     & /raptor\_dbw\_interface/pt\_report & Output & & \\
     & /raptor\_dbw\_interface/misc\_report\_do & Output & & \\
    \hline
\end{tabular}
\caption{\label{table:communication_module}Communication Module inputs and outputs.}
\end{table*}

\begin{table*}[p]
\begin{tabular}{c|c|c|c|c}
    \textbf{Node} & \textbf{Topic} & \textbf{I/O Type} & \textbf{Failure Type} & \textbf{HALO Safety Node} \\
    \hline
    LiDAR Front & /luminar\_front\_points & Output & & \\
    \hline
    LiDAR Left & /luminar\_left\_points & Output & & \\
    \hline
    LiDAR Right & /luminar\_right\_points & Output & & \\
    \hline
    Point Cloud Transformer Front & /luminar\_front\_points & Input & & \\
     & /luminar\_front\_points/filtered & Output & & \\
    \hline
    Point Cloud Transformer Left & /luminar\_left\_points & Input & & \\
     & /luminar\_left\_points/filtered & Output & & \\
    \hline
    Point Cloud Transformer Right & /luminar\_right\_points & Input & & \\
     & /luminar\_right\_points/filtered & Output & & \\
    \hline
    LiDAR Fusion & /luminar\_front\_points/filtered & Input & & \\
     & /luminar\_left\_points/filtered & Input & & \\
     & /luminar\_right\_points/filtered & Input & & \\
     & /points\_fused & Output & & \\
    \hline
    Ray Ground Classifier & /points\_fused & Input & & \\
     & /points\_ground & Output & & \\
     & /points\_nonground & Output & & \\
    \hline
    Right Wall Detector & /novatel\_top/dyntf\_odom & Input & Data Health & Topic Multiplexer \\
     & /points\_ground & Input & & \\
     & /points\_nonground & Input & & \\
     & /real\_points & Output & & \\
     & /right\_wall & Output & & \\
     & /left\_wall & Output & & \\
    \hline
    Euclidean Cluster & /real\_points & Input & & \\
     & /lidar\_bounding\_boxes & Output & & \\
    \hline
    Right Wall Points Pub & /right\_wall & Input & & \\
     & /points\_right\_wall & Output & & \\
     & /path\_right\_wall & Output & & \\
    \hline
    Left Wall Points Pub & /left\_wall & Input & & \\
     & /points\_left\_wall & Output & & \\
     & /path\_left\_wall & Output & & \\
    \hline
    Heading Estimator & /lidar\_bounding\_boxes & Input & & \\
     & /novatel\_top/dyntf\_odom & Input & Data Health & Topic \\
     & /telemetry/bounding\_box\_array & Output & & \\
     & /telemetry/bb\_distance & Output & Behavioral-Safety & SSC Interface \\
    \hline
\end{tabular}
\caption{\label{table:perception_module}Perception Module inputs and outputs.}
\end{table*}
